# Supplementary material for: Incorporating compositional heterogeneity into Lie Markov models for phylogenetic inference
Source: arXiv:2007.08511 ancillary file (2020-07-17)
Supplement: Supplementary file 1 [file supplMat.pdf]

# Supplementary Material for "Incorporating compositional heterogeneity into Lie Markov models for phylogenetic inference"

Naomi E. Hannaford[1], Sarah E. Heaps[1,*], Tom M. W. Nye[1], Tom A. Williams[2] and T. Martin Embley[3]

[1]School of Mathematics, Statistics and Physics, Newcastle University, Newcastle upon Tyne, U.K.
[2]School of Biological Sciences, University of Bristol, Bristol, U.K.
[3]Institute for Cell and Molecular Biosciences, Newcastle University, Newcastle upon Tyne, U.K.
[*]Corresponding author: sarah.heaps@ncl.ac.uk

# S1 Lie Markov models – stationary distribution

## S1.1 RY5.6b model

As discussed in Section 3.1 of the main text, there is a strong positive relationship between the simplex-valued parameters $\boldsymbol{\rho}$ in the RY5.6b model and the corresponding stationary distribution $\boldsymbol{\pi}$. To demonstrate this numerically, we simulate a sample of $\boldsymbol{\rho}$ vectors from a uniform distribution over $\mathscr{S}_4$ and then compute the corresponding stationary distribution $\boldsymbol{\pi}$ for various values of $\alpha$. This is illustrated in Figure S1 which shows plots of $\pi_i$ against $\rho_i$.

## S1.2 RY8.8a model

In Section 3.2 of the main text, we showed that the RY8.8a model can be parameterised in terms of a single stochastic vector $\boldsymbol{\rho} \in \mathscr{S}_8$. It is then straightforward to verify that the analytic forms for the stationary probabilities in $\boldsymbol{\pi}$ are given by

$$\pi_1 = \frac{(2\rho_1 + \rho_7 + \rho_8)\rho_5 + 2\rho_1\rho_6}{k_1 k_2}, \qquad \pi_2 = \frac{(2\rho_2 + \rho_7 + \rho_8)\rho_6 + 2\rho_2\rho_5}{k_1 k_2},$$
$$\pi_3 = \frac{(2\rho_3 + \rho_5 + \rho_6)\rho_7 + 2\rho_3\rho_8}{k_2 k_3}, \qquad \pi_4 = \frac{(2\rho_4 + \rho_5 + \rho_6)\rho_8 + 2\rho_4\rho_7}{k_2 k_3},$$

where

$$k_1 = \rho_8 + 2\rho_2 + \rho_7 + 2\rho_1, \quad k_2 = \rho_5 + \rho_6 + \rho_7 + \rho_8, \quad k_3 = 2\rho_3 + 2\rho_4 + \rho_5 + \rho_6.$$

# S2 Analysis of simulated data

## S2.1 Different numbers of taxa and sites

In Section 6.1 of the main text, we consider the effect on inference of varying the number of sites and taxa in the alignment. Three values are considered for the number of taxa (6, 12, 24) and for the number of sites (500, 1000 and 2000). The trees used to simulate the data are shown in Figure S2. In the main text, the left-hand panels of Figure 2 show the posterior distribution over root splits for the alignments simulated and analysed under the non-homogeneous RY5.6b model. The right-hand panels show the corresponding distributions for the non-homogeneous RY8.8a model. The analogous plots displaying the posterior distribution over unrooted topologies is shown in Figure S3.

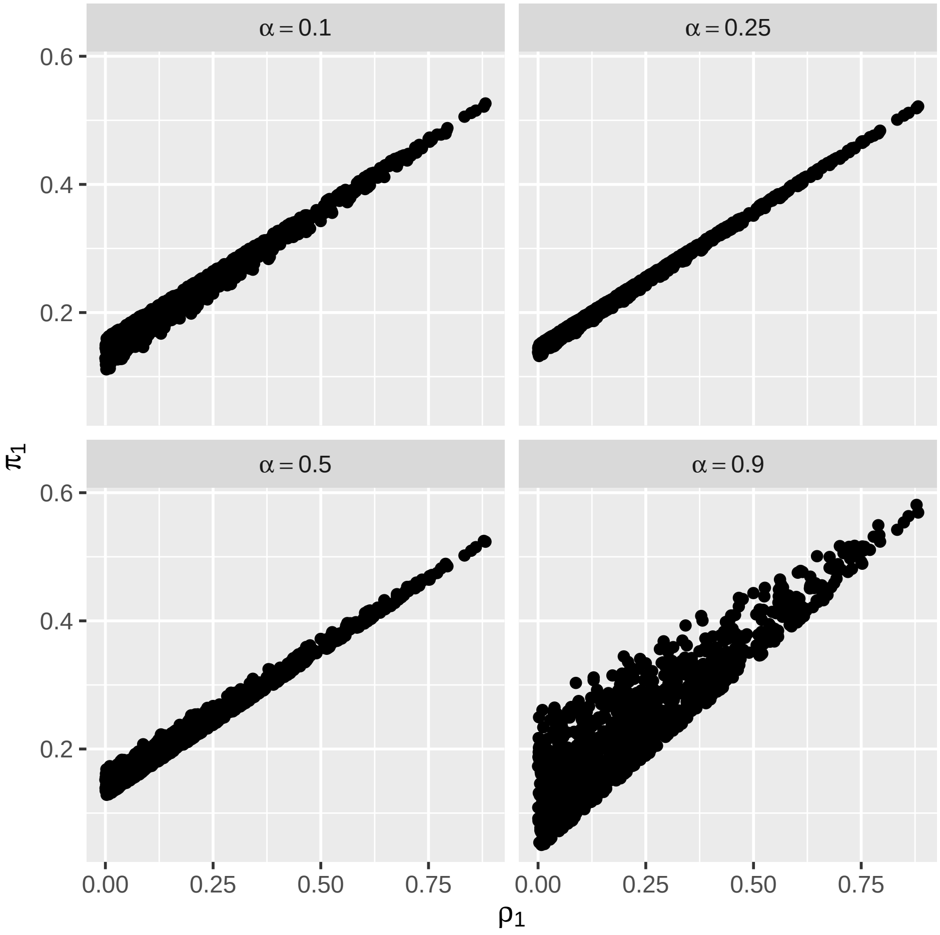


Figure S1: Plots of the stationary probability $\pi_1$ of the RY5.6b model against $\rho_1$ for values of $\boldsymbol{\rho}$ sampled from the uniform distribution over $\mathscr{S}_4$ and various values of $\alpha$. By symmetry, plots for the other pairs $(\rho_i, \pi_i)$, $i = 2, 3, 4$, displayed identical patterns and are not shown.

The non-homogeneous Lie Markov models are, by design, highly parameterised. Although of secondary interest in its own right, identifiability of the quantitative model parameters in the posterior is likely to impact on inference of the root position and topology. In the most highly parameterised case, where data are simulated under a 24-taxon tree, we therefore investigated the extent to which the true values of the model parameters could be identified in the posterior. For one of the three alignments, results are summarised in Figures S4 and S5 for the non-homogeneous RY5.6b and RY8.8a models, respectively, and show the effect of varying the number of sites from 500 through 1000 to 2000. Results for the other two alignments showed the same patterns and are not shown. The posterior densities for the global parameters $\phi$, in the discretised gamma distribution for rate variation across sites, and $\alpha$, from the RY5.6b rate matrix, are based on draws from the joint posterior of all unknowns. The branch lengths $\ell_1, \ldots, \ell_B$ and branch-specific parameter vectors $\boldsymbol{\rho}_1, \ldots, \boldsymbol{\rho}_{B-1}$ are only meaningfully labelled on the tree in Figure S2c used to simulate the data, say $\tau_{\text{true}}$. The densities for the branch-specific parameters are therefore based on draws from the conditional posterior of the model parameters given the topology $\tau = \tau_{\text{true}}$. Posterior densities are visualised for a representative, random selection of branch-specific parameters.

For both models, the true values of the global parameters and branch lengths are identified with high posterior support, even with only 500 sites in the alignment. In nearly all cases, the true values of the branch-specific $\rho_{bk}$ lie within the main body of the posterior density, and the posterior becomes more concentrated around the true value as the number of sites in

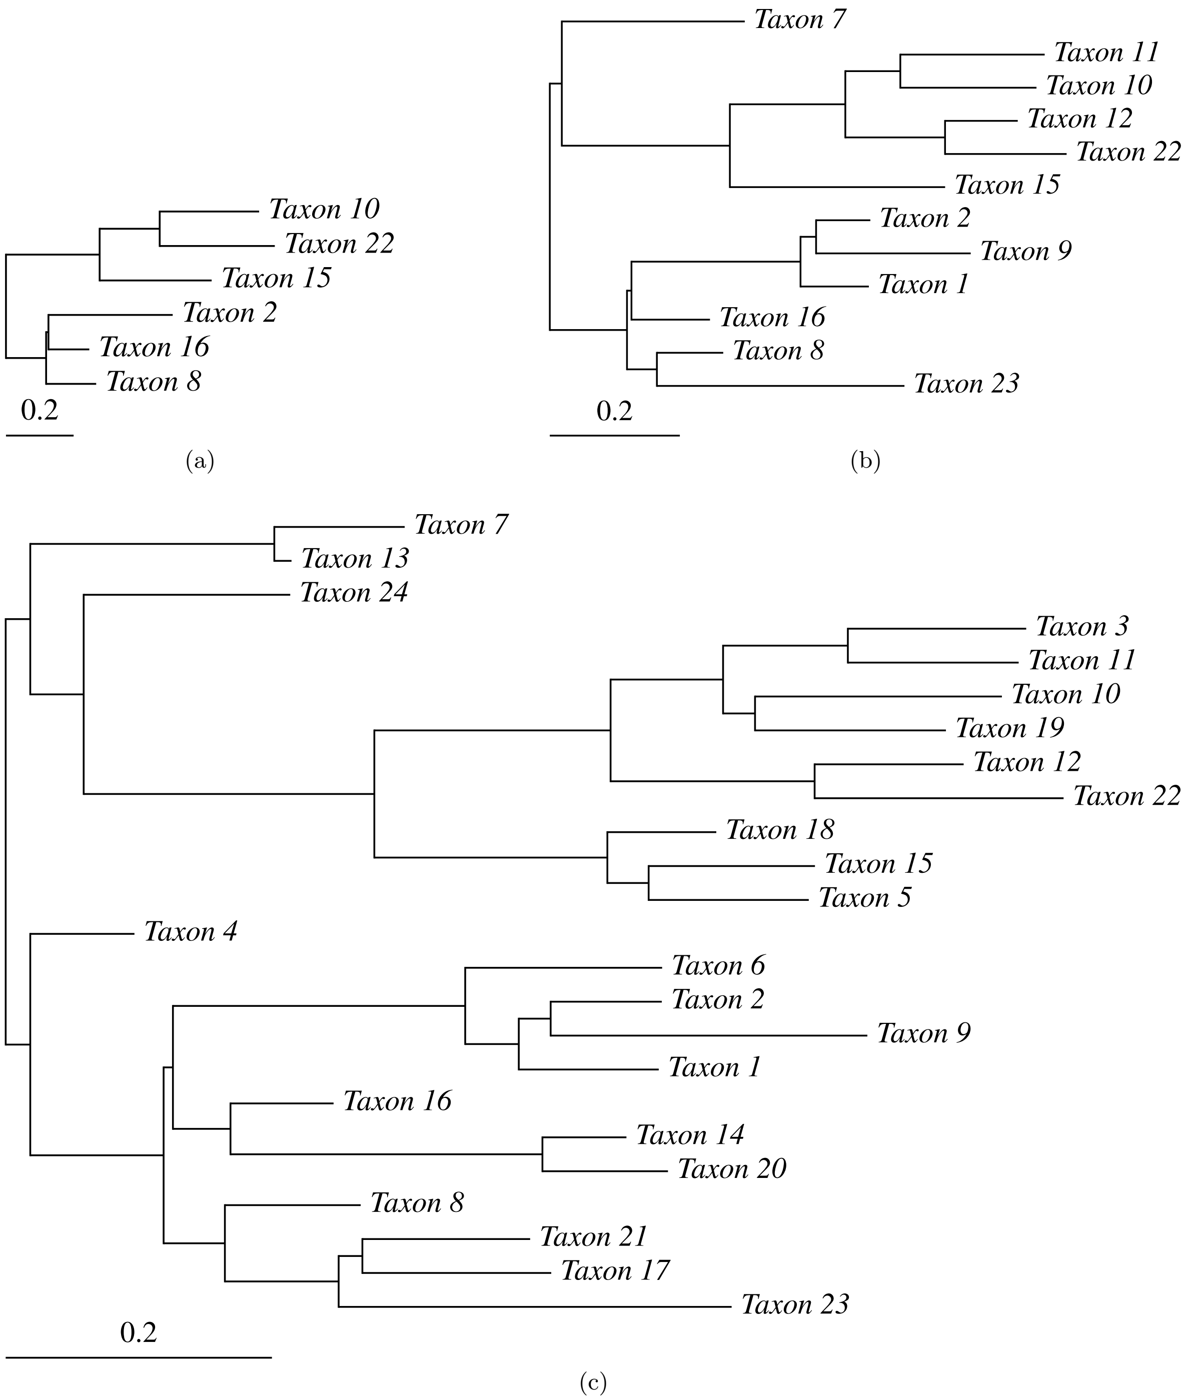


Figure S2: Trees used to simulate alignments on (a) 6, (b) 12, (c) 24 taxa.

the alignment increases. However, it is clear that the posteriors for the $\rho_{bk}$ are much more concentrated under the non-homogeneous RY8.8a model than the RY5.6b model. This may be because the additive structure of the RY5.6b rate matrix makes the likelihood less sensitive to changes in the $\boldsymbol{\rho}_b$ and is likely to be partly responsible for the poorer rooting performance of the non-homogeneous RY5.6b model.

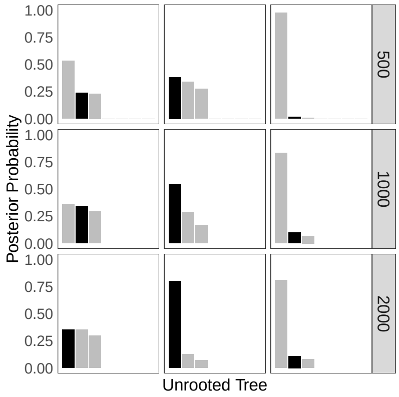


(a)

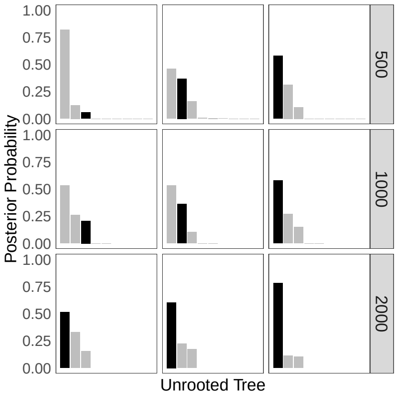


(b)

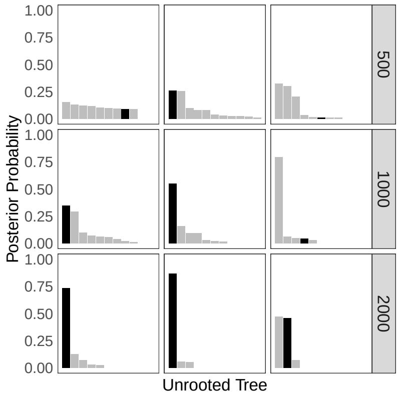


(c)

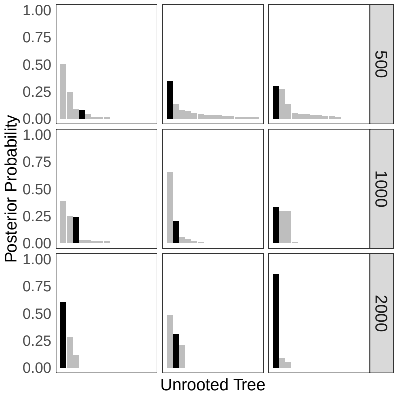


(d)

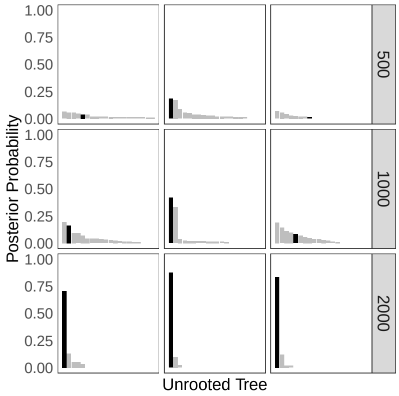


(e)

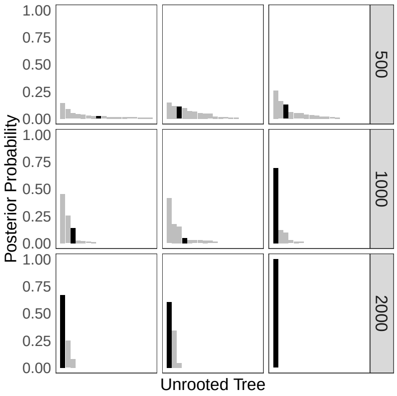


(f)

Figure S3: Posterior distribution over unrooted topologies when the data are simulated and analysed under the non-homogeneous RY5.6b model and the number of taxa is (a) 6, (c) 12, (e) 24; and when the data are simulated and analysed under the non-homogeneous RY8.8a model and the number of taxa is (b) 6, (d) 12, (f) 24. Highlighted in black is the correct unrooted topology. In the plots for 12 and 24 taxa, bars corresponding to probabilities less than 0.01 have been removed to improve readability.

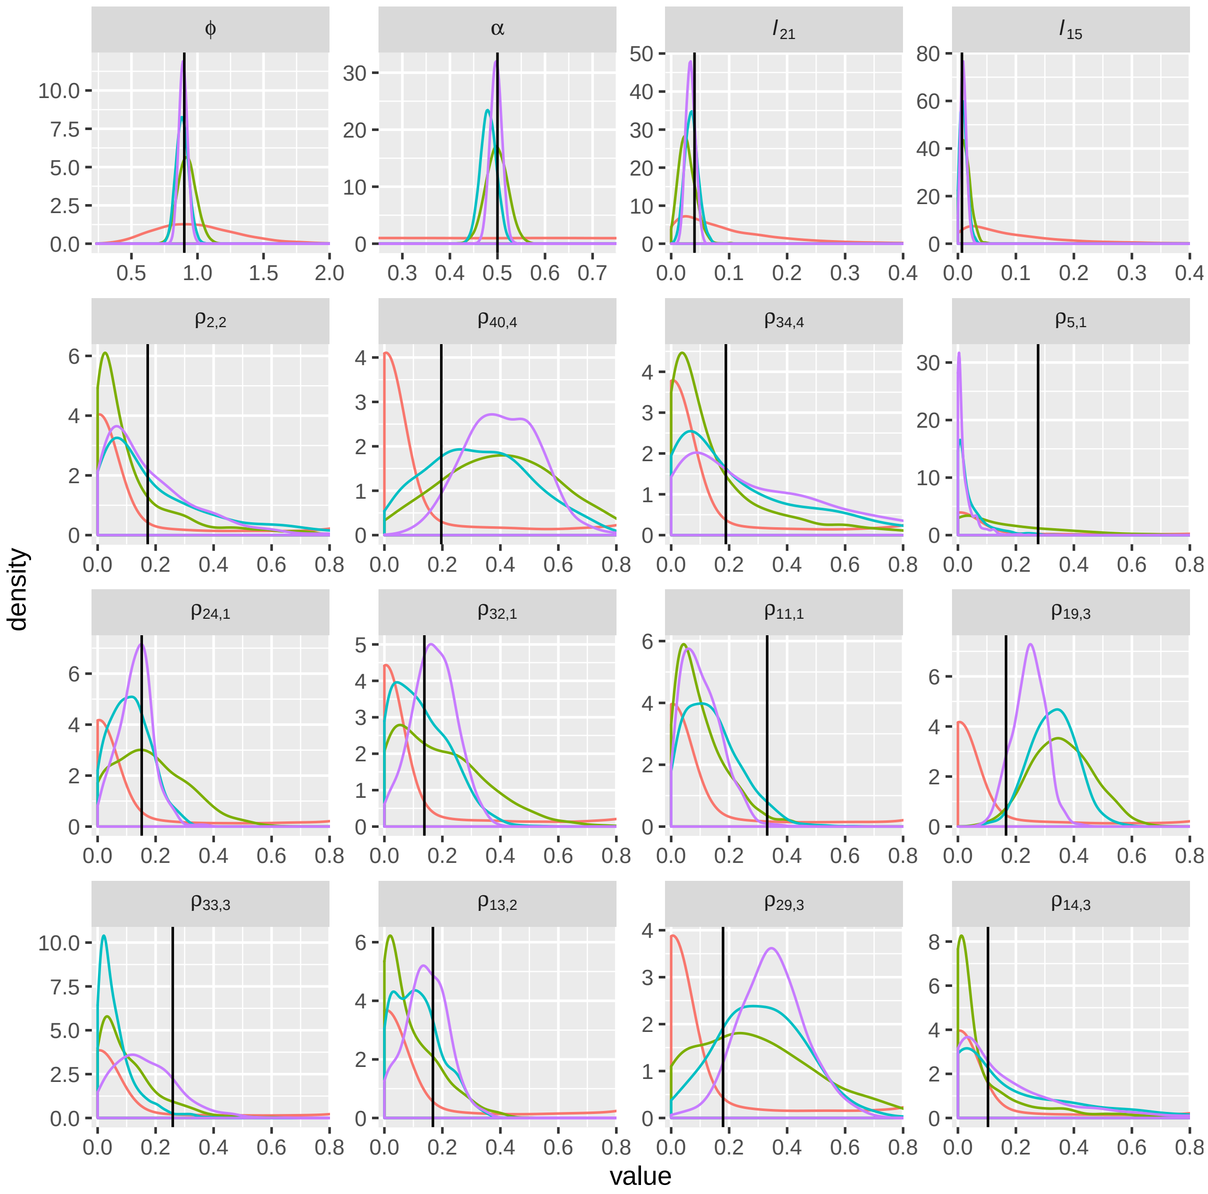


Figure S4: Marginal prior and posterior densities for the global model parameters ($\phi$ and $\alpha$) and a random sample of branch-specific parameters in the analysis of a 24-taxon alignment simulated under the non-homogeneous RY5.6b model. Posterior densities for the branch-specific parameters are conditional on the rooted topology used to simulate the data. Indicated in the panels are the prior (—) and posterior when the number of sites is 500 (—), 1000 (—) and 2000 (—). The true values of the parameters are indicated by vertical lines.

## S2.2 Different topologies and branch lengths

Section 6.2 of the main text considers the effect on inference of prior-data conflict that can arise when there is a long branch in the unrooted tree or the rooted topology is unbalanced. In the main text, Figure 4 shows the posterior over root splits for alignments simulated and analysed under the non-homogeneous RY8.8a model. The corresponding plots for the non-homogeneous RY5.6b model are displayed in Figure S6.

Analogous plots displaying the posterior distribution over unrooted topologies are shown in Figures S7 and S8 for the non-homogeneous RY5.6b and RY8.8a models, respectively.

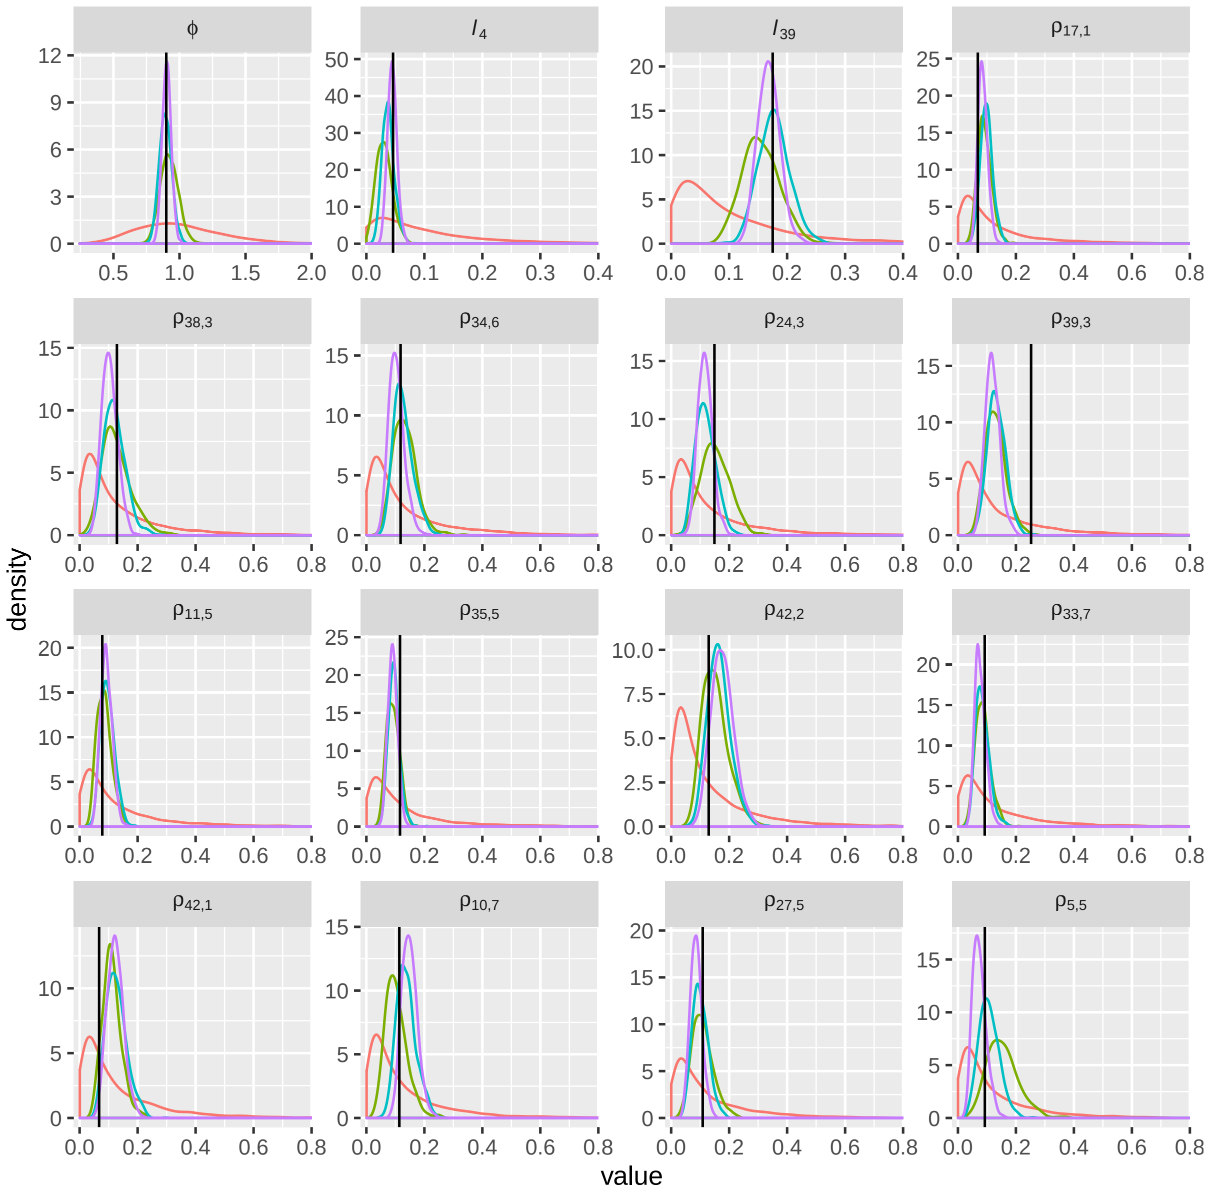


Figure S5: Marginal prior and posterior densities for the global model parameter ($\phi$) and a random sample of branch-specific parameters in the analysis of a 24-taxon alignment simulated under the non-homogeneous RY8.8a model. Posterior densities for the branch-specific parameters are conditional on the rooted topology used to simulate the data. Indicated in the panels are the prior (—) and posterior when the number of sites is 500 (—), 1000 (—) and 2000 (—). The true values of the parameters are indicated by vertical lines.

# S3 Application

## S3.1 Prior specification

In the *Drosophila* application, we adopt the prior described in Section 6 of the main text for the non-homogeneous Lie Markov models, $\mathcal{M}_5$ and $\mathcal{M}_6$. For models $\mathcal{M}_i$, $i = 1, \ldots, 4$, the unknowns comprise the tree topology $\tau$, branch lengths $\boldsymbol{\ell} = (\ell_1, \ldots, \ell_B)^T \in \mathbb{R}_+^B$, substitution model parameters $\mathcal{Q}_i$ for model $i$ and the shape parameter $\phi \in \mathbb{R}_+$ in the discretised gamma distribution for rate variation across sites. For model $\mathcal{M}_1$, $\tau$ belongs to the set $\mathcal{U}_n$ of unrooted tree topologies on $n$ species and there are $B = 2n-3$ branches. For models $\mathcal{M}_2 - \mathcal{M}_4$, $\tau$ belongs

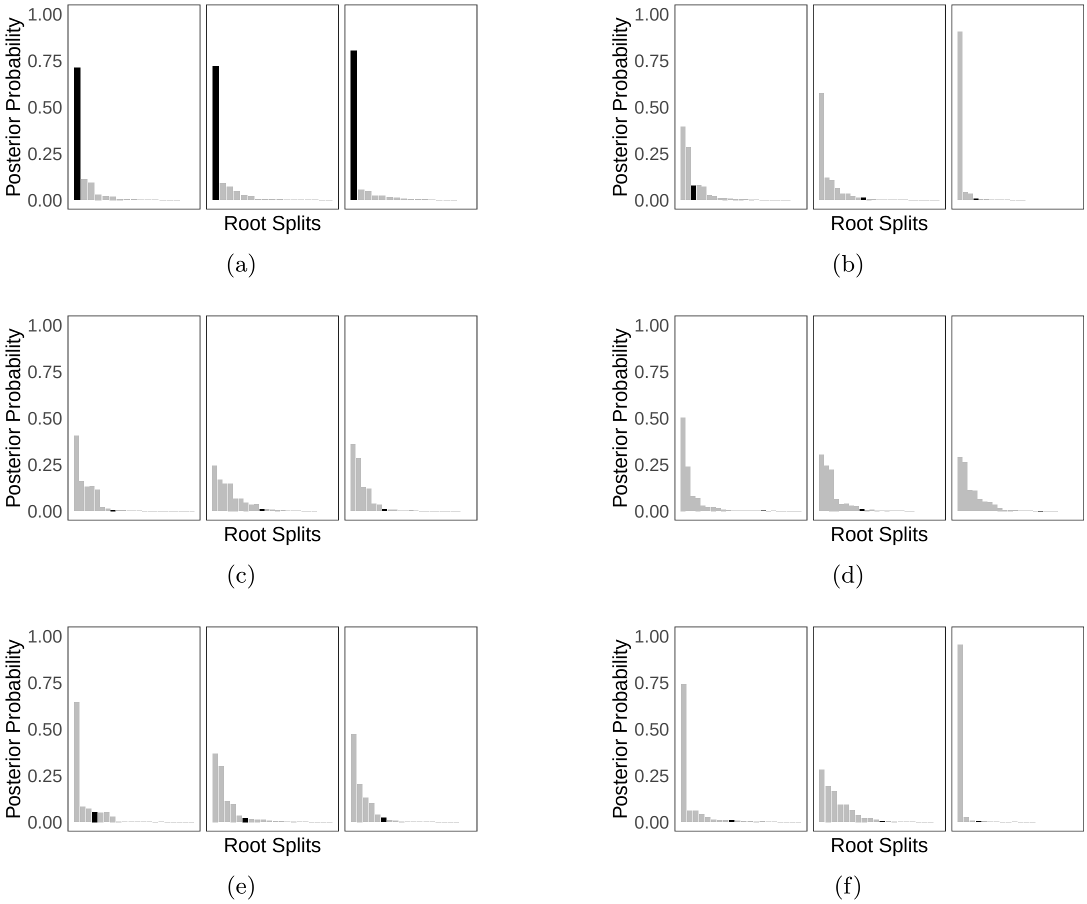


Figure S6: Posterior distribution over roots splits when three data sets are simulated and analysed under the non-homogeneous RY5.6b model and the tree used for simulation is Tree (a) 1 (balanced, long root branch), (b) 2 (unbalanced, long internal branch), (c) 3 (balanced, short root branch), (d) 4 (unbalanced, short internal branch), (e) 5 (balanced, medium root branch), (f) 6 (unbalanced, medium internal branch). In every plot, bars are arranged in descending order of posterior probability and the correct root split is highlighted in black.

to the set of rooted tree topologies on $n$ species and there are $B = 2n - 2$ branches.

As for models $\mathcal{M}_5$ and $\mathcal{M}_6$, our prior takes the form $\pi(\tau, \boldsymbol{\ell}, \phi, \mathcal{Q}_i) = \pi(\tau)\pi(\phi)\pi(\mathcal{Q}_i|\tau)\prod_{b=1}^{B}\pi(\ell_b)$ for model $\mathcal{M}_i$, where the dependence of $\mathcal{Q}_i$ on $\tau$ is dropped for the homogeneous models $\mathcal{M}_1 - \mathcal{M}_3$. In keeping with standard practice in the phylogenetics literature, we assign priors $\ell_b \sim \text{Exp}(10)$ to the branch lengths, expressing the belief that there will be $\text{E}(\ell_b) = 0.1$ substitutions per site on average. For the shape parameter we assign $\phi \sim \text{Ga}(10, 10)$ to give a distribution which is modestly concentrated about $\text{E}(\phi) = 1$, conveying the belief that the multiplicative random effects across sites will equal 1 on average. For models $\mathcal{M}_2 - \mathcal{M}_4$ we assign the rooted topology a Yule prior and for the GTR model $\mathcal{M}_1$ we assign the unrooted topology a prior which is uniform over $\mathcal{U}_n$, expressing prior indifference with respect to the topology.

The substitution model parameters $\mathcal{Q}_1$ in $\mathcal{M}_1$ comprise the theoretical stationary distribution $\boldsymbol{\pi} \in \mathscr{S}_4$ and the exchangeability parameters $\boldsymbol{\kappa} = (\kappa_{12}, \kappa_{13}, \kappa_{14}, \kappa_{23}, \kappa_{24})^T \in \mathbb{R}_+^5$ to which we assign the prior

$$\pi(\mathcal{Q}_1) = \pi(\boldsymbol{\pi}) \prod_{i=1}^{2} \prod_{j=i+1}^{4} \pi(\kappa_{ij}) \quad \text{where} \quad \boldsymbol{\pi} \sim \mathscr{D}_4(1,1,1,1), \quad \kappa_{ij} \sim \text{Ga}(1,1).$$

In the homogeneous RY5.6b model $\mathcal{M}_2$, the substitution model parameters consist of the stochas-

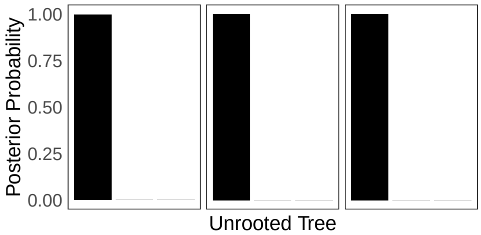


(a)

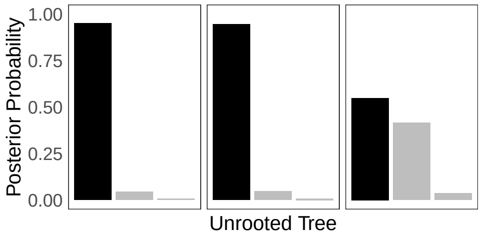


(b)

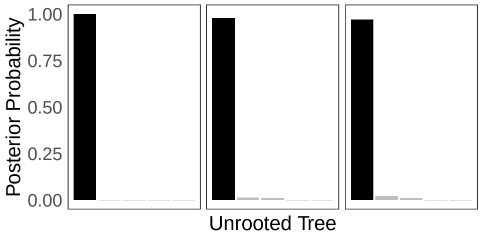


(c)

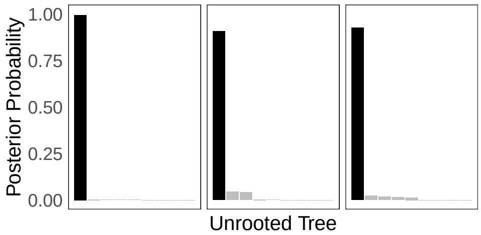


(d)

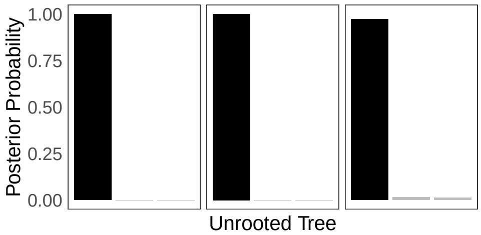


(e)

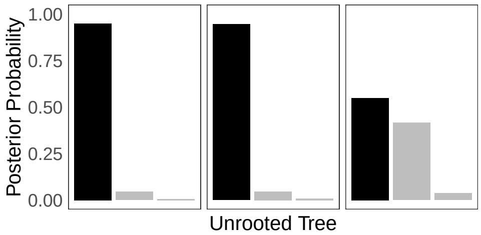


(f)

Figure S7: Posterior distribution over unrooted topologies when three data sets are simulated and analysed under the non-homogeneous RY5.6b model and the tree used for simulation is Tree (a) 1 (balanced, long root branch), (b) 2 (unbalanced, long internal branch), (c) 3 (balanced, short root branch), (d) 4 (unbalanced, short internal branch), (e) 5 (balanced, medium root branch), (f) 6 (unbalanced, medium internal branch). In every plot, bars are arranged in descending order of posterior probability and the correct unrooted topology is highlighted in black.

tic vector $\boldsymbol{\rho} \in \mathscr{S}_4$, which controls the theoretical stationary distribution, and the parameter $\alpha \in \mathbb{R}_+$. We assign the prior

$$\pi(\mathcal{Q}_2) = \pi(\boldsymbol{\rho})\pi(\alpha) \quad \text{where} \quad \boldsymbol{\rho} \sim \mathscr{D}_4(1,1,1,1), \quad \alpha \sim \text{Beta}(1,1).$$

For the homogeneous RY8.8a model $\mathcal{M}_3$, the substitution model parameters simply comprise the stochastic vector $\boldsymbol{\rho} \in \mathscr{S}_8$ and we assign the prior $\boldsymbol{\rho} \sim \mathscr{D}_8(\mathbf{1}_8)$, where $\mathbf{1}_n$ denotes an $n$-vector of 1s.

For the non-homogeneous GTR model $\mathcal{M}_4$, the substitution model parameters $\mathcal{Q}_4$ comprise the branch-specific composition vectors $\boldsymbol{\pi}_b \in \mathscr{S}_4$ for $b = 1, \ldots, B-1$ and the shared set of GTR exchangeability parameters $\boldsymbol{\kappa} = (\kappa_{12}, \kappa_{13}, \kappa_{14}, \kappa_{23}, \kappa_{24})^T \in \mathbb{R}_+^5$. We assign the prior

$$\pi(\mathcal{Q}_4|\tau) = \pi(\boldsymbol{\pi}_1, \ldots, \boldsymbol{\pi}_{B-1}|\tau) \prod_{i=1}^{2} \prod_{j=i+1}^{4} \pi(\kappa_{ij})$$

in which $\kappa_{ij} \sim \text{Ga}(1,1)$ and the $\boldsymbol{\pi}_b$ are assigned the same joint, conditional distribution as the $\boldsymbol{\rho}_b$; see Section 4 of the main text.

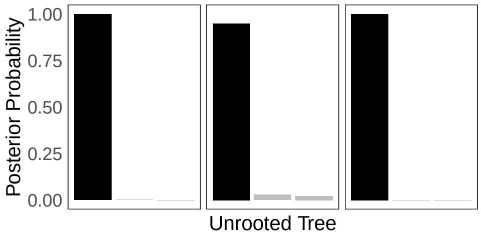


(a)

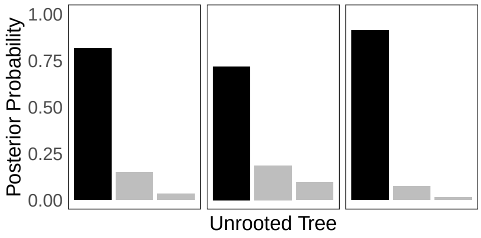


(b)

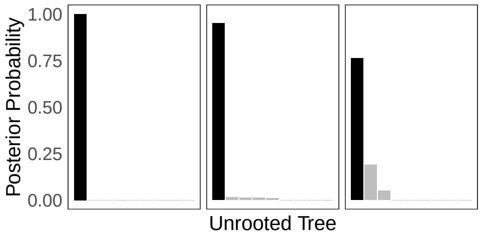


(c)

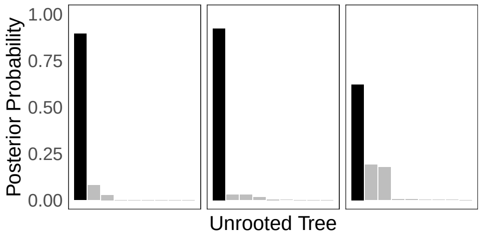


(d)

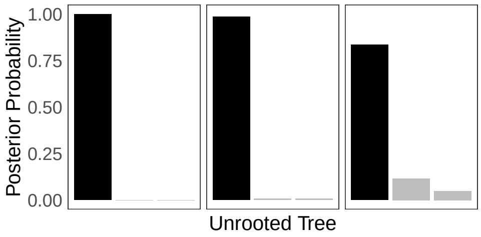


(e)

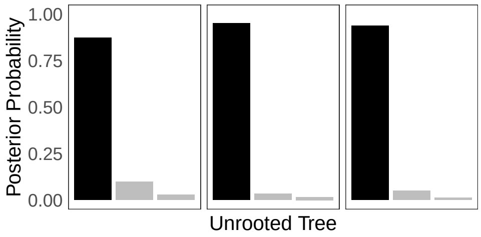


(f)

Figure S8: Posterior distribution over unrooted topologies when three data sets are simulated and analysed under the non-homogeneous RY8.8a model and the tree used for simulation is Tree (a) 1 (balanced, long root branch), (b) 2 (unbalanced, long internal branch), (c) 3 (balanced, short root branch), (d) 4 (unbalanced, short internal branch), (e) 5 (balanced, medium root branch), (f) 6 (unbalanced, medium internal branch). In every plot, bars are arranged in descending order of posterior probability and the correct unrooted topology is highlighted in black.

The choices of the parameters $p_\varrho$ and $v_\varrho$ in our priors for the branch-specific simplex-valued parameters in models $\mathcal{M}_4 - \mathcal{M}_6$ are:

$$\begin{aligned} \mathcal{M}_4: &\quad p_\varrho = 0.94, \quad v_\varrho = 0.31^2; \\ \mathcal{M}_5: &\quad p_\varrho = 0.95, \quad v_\varrho = 2.00^2; \\ \mathcal{M}_6: &\quad p_\varrho = 0.94, \quad v_\varrho = 0.38^2. \end{aligned}$$

For the non-homogeneous GTR model $\mathcal{M}_4$, our method for choosing the hyperparameters is described in detail in (Heaps et al., 2014). In brief, this involves a process of trial-and-improvement, varying $p_\varrho$ and $v_\varrho$ until samples from the ensuing prior predictive distribution of the empirical sequence composition matches quantiles informed by expert biological judgement. For the non-homogeneous Lie Markov models, $\mathcal{M}_5$ and $\mathcal{M}_6$, we adopted the same iterative procedure.

## S3.2 Relative computational times

Taking as a baseline, the computational time to run a fixed number of MCMC iterations for model $\mathcal{M}_1$ (i.e. the homogeneous, stationary and reversible GTR model), the computational times for the homogeneous, non-reversible RY5.6b and RY8.8a models, $\mathcal{M}_2$ and $\mathcal{M}_3$, are broadly

consistent with this time across a range of alignment sizes. The computational times for the three non-homogeneous models, $\mathcal{M}_4$, $\mathcal{M}_5$ and $\mathcal{M}_6$, are broadly consistent with each other and around double the times for the homogeneous models, $\mathcal{M}_1$, $\mathcal{M}_2$ and $\mathcal{M}_3$. The length of the alignment has a linear effect on the computation times whilst the number of taxa seems to have a superlinear effect for all models; for example, doubling the number of taxa from 6 to 12 increases the computation times by a factor of around 2.7, whilst doubling the number of taxa again from 12 to 24 increases the computation time by a factor of around 2.4.

## S3.3 Model comparison

Many techniques for approximating the marginal likelihood are based on importance sampling or reciprocal importance sampling. For the *Drosophila* application, these methods would use the identities

$$p(y|\mathcal{M}_i) = \mathrm{E}_q\left\{\frac{p(y|\tau,\Theta_i,\mathcal{M}_i)\pi(\tau,\Theta_i|\mathcal{M}_i)}{q(\tau,\Theta_i|\mathcal{M}_i)}\right\}, \tag{1}$$

or

$$p(y|\mathcal{M}_i) = \left[\mathrm{E}_\pi\left\{\frac{q(\tau,\Theta_i|\mathcal{M}_i)}{p(y|\tau,\Theta_i,\mathcal{M}_i)\pi(\tau,\Theta_i|\mathcal{M}_i)}\right\}\right]^{-1}, \tag{2}$$

where $\mathrm{E}_q$ and $\mathrm{E}_\pi$ denote expectation with respect to the importance density $q(\tau,\Theta_i|\mathcal{M}_i)$ and the posterior $\pi(\tau,\Theta_i|y,\mathcal{M}_i)$, respectively. Taking $q(\tau,\Theta_i|\mathcal{M}_i)$ to be the prior $\pi(\tau,\Theta_i|\mathcal{M}_i)$ in (1) and (2) leads to the widely used Monte Carlo and harmonic mean estimators, respectively. The main advantages of these techniques are their computational simplicity, requiring only a sample from the prior in the former case, or posterior in the latter case. However, both are prone to large Monte Carlo error, essentially because the prior and posterior are generally very different, with the former being substantially more diffuse. Motivated by this observation, a number of techniques have been developed that build up the approximation using sequences of intermediate densities that form a bridge between the prior and posterior. Methods that have received considerable attention in the phylogenetic literature are thermodynamic integration (Lartillot and Philippe, 2006), also called the power posterior approach (Friel and Pettitt, 2008), and the stepping-stone method (Xie et al., 2011). The problem with these methods is that they require samples from each of the intermediate densities and so implementation of the algorithms is highly computationally expensive. Indeed, we have found them to be practically infeasible for the more complex non-homogeneous models introduced here.

In an effort to stabilise the variance of the harmonic mean estimator, Newton and Raftery (1994) suggested a hybrid estimator, based on combined samples from the prior and posterior. In practice, it has been found to perform better than the Monte Carlo or harmonic mean estimators (Green, 2003). Starting with the simulation consistent marginal likelihood estimator

$$\frac{\sum_{m=1}^{M} \pi(\tau^{[m]},\Theta_i^{[m]}|\mathcal{M}_i)/q(\tau^{[m]},\Theta_i^{[m]}|\mathcal{M}_i) \times p(y|\tau^{[m]},\Theta_i^{[m]},\mathcal{M}_i)}{\sum_{m=1}^{M} \pi(\tau^{[m]},\Theta_i^{[m]}|\mathcal{M}_i)/q(\tau^{[m]},\Theta_i^{[m]}|\mathcal{M}_i)}$$

and taking the importance density to be

$$q(\tau,\Theta_i|\mathcal{M}_i) = \delta\pi(\tau,\Theta_i|\mathcal{M}_i) + (1-\delta)\pi(\tau,\Theta_i|y,\mathcal{M}_i),$$

with $0 < \delta < 1$ and $\delta$ small, leads to the approximation

$$\hat{p}(y|\mathcal{M}_i) = \frac{\sum_{m=1}^{M} \frac{p(y|\tau^{[m]},\Theta_i^{[m]},\mathcal{M}_i)}{\delta\hat{p}(y|\mathcal{M}_i) + (1-\delta)p(y|\tau^{[m]},\Theta_i^{[m]},\mathcal{M}_i)}}{\sum_{m=1}^{M} \{\delta\hat{p}(y|\mathcal{M}_i) + (1-\delta)p(y|\tau^{[m]},\Theta_i^{[m]},\mathcal{M}_i)\}^{-1}},$$

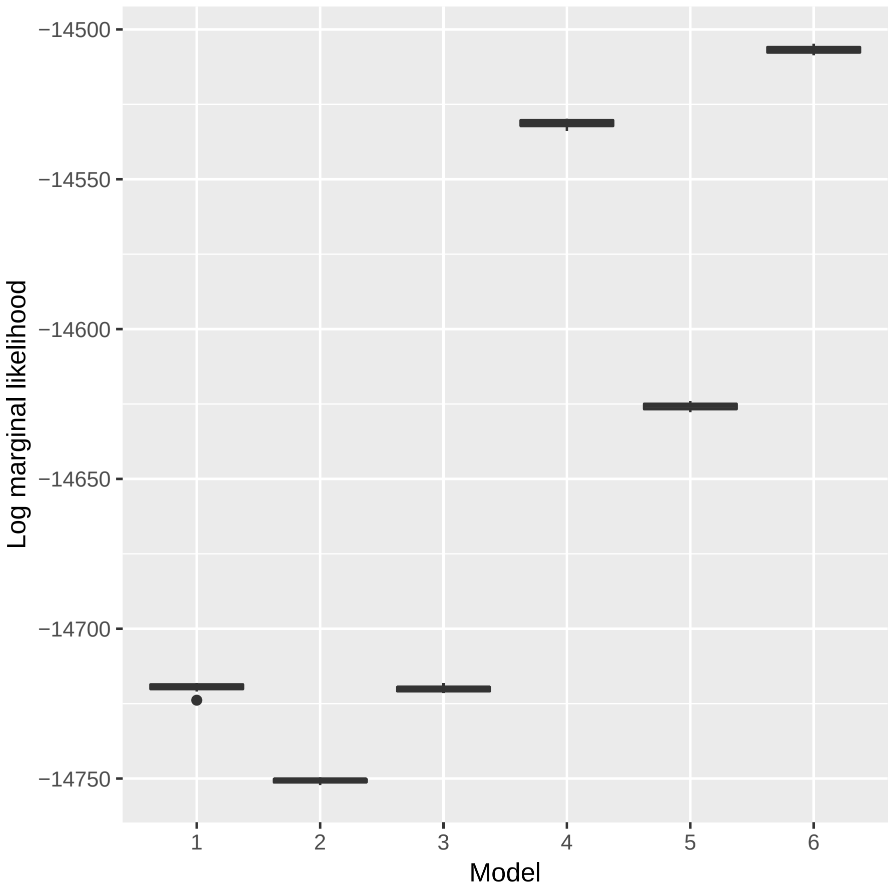


Figure S9: Box-plots of the Newton and Raftery hybrid estimates of the marginal likelihood for each model $\mathcal{M}_i$, $i = 1, \ldots, 6$, based on the output of 10 MCMC chains which were initialised at different starting points.

which can be computed by a standard iterative scheme using draws $(\tau^{[m]}, \Theta_i^{[m]})$, $m = 1, \ldots, M$, from $q(\tau, \Theta_i|\mathcal{M}_i)$.

For models $\mathcal{M}_1 - \mathcal{M}_6$ in the *Drosophila* application, the log marginal likelihoods obtained using the Newton and Raftery hybrid estimator (with $\delta = 0.05$) are displayed in Table 1 of the main text. It is reassuring to note that although the numerical values of the approximations differed, the Monte Carlo and harmonic mean estimators produced the same ranking of the non-homogeneous models.

Although the Newton and Raftery hybrid estimator tends to be more stable than the harmonic mean estimator (Newton and Raftery, 1994), its variance can still be large. For each of the models $\mathcal{M}_1 - \mathcal{M}_6$, we therefore ran ten MCMC chains, initialised at different starting points, and repeated the calculation of the marginal likelihood. The results are summarised in Figure S9, where the box-plots for the homogeneous and non-homogeneous models are well separated and similarly for the three non-homogeneous models $\mathcal{M}_4 - \mathcal{M}_6$. Even after allowing for Monte Carlo error, therefore, these results do not give any cause to question the ranking of models, and subsequent conclusions, drawn in the paper.

## References

Friel, N. and A. N. Pettitt (2008). Marginal likelihood estimation via power posteriors. *Journal of the Royal Statistical Society: Series B 70*, 589–607.

Green, P. J. (2003). Trans–dimensional Markov chain Monte Carlo. In P. J. Green, N. L. Hjort, and S. Richardson (Eds.), *Highly Structured Stochastic Systems*, Volume 27 of *Oxford Statist. Sci. Ser.*, pp. 179–206. Oxford: Oxford Univ. Press.

Heaps, S. E., T. M. W. Nye, R. J. Boys, T. A. Williams, and T. M. Embley (2014). Bayesian modelling of compositional heterogeneity in molecular phylogenetics. *Statistical Applications in Genetics and Molecular Biology 1*, 1–21.

Lartillot, N. and H. Philippe (2006). Computing Bayes factors using thermodynamic integration. *Systematic Biology 55*, 195–207.

Newton, M. A. and A. E. Raftery (1994). Approximate Bayesian inference by the weighted likelihood bootstrap (with discussion). *Journal of the Royal Statistical Society: Series B 56*, 3–48.

Xie, W., P. O. Lewis, Y. Fan, L. Kuo, and M.-H. Chen (2011). Improving marginal likelihood estimation for Bayesian phylogenetic model selection. *Systematic Biology 60*, 150–160.
